# Supplementary material for: CHIMERA: Adaptive Cache Injection and Semantic Anchor Prompting for Zero-shot Image Morphing with Morphing-oriented Metrics
Source: arXiv:2512.07155 source file (2026-10-10)
Supplement: Supplementary file 1 [file X_suppl_freq_analysis.tex]

% \begin{figure}
%     \centering
%     \includegraphics[width=1.0\textwidth]{./figs/another_backbone_freq_analysis.pdf}
%     \caption{\textbf{Frequency analysis on another backbone.} (i) and (iii) show the layer-wise frequency characteristics of a given diffusion model, while (ii) and (iv) present the timestep-wise frequency characteristics. In each plot, the orange line represents high-frequency components and the blue line represents low-frequency components.}
%     \label{fig:another_backbone_freq} 
% \end{figure}


% \section{Further Analysis on Another Backbone}\label{sp_sec:freq_analysis}

% In this section, we provide additional analyses for the experiments presented in \cref{exp:further_analysis}. 
% In \cref{Sec:PreNObs}, we analyzed diffusion features from a frequency perspective and presented observations that motivate adaptive feature injection based on layer-wise and timestep-wise characteristics. 
% Here, we extend the same frequency-based analysis to other diffusion models to demonstrate that CHIMERA with ACI can generalize to different architectures.

% The analysis in \cref{fig:freq_analysis} focuses on layer- and timestep-wise characteristics of SD~2.1~\cite{rombach2022high}. 
% In this section, we extend the analysis to other U-Net-based diffusion models, including SD~1.4, SD~1.5, and SD~2, as well as larger models such as SDXL~\cite{podell2023sdxl} and the DiT-based model FLUX~\cite{peebles2023scalable,labs2025flux}. 
% As shown in \cref{fig:another_backbone_freq}~(a)-(c), U-Net-based diffusion models share very similar layer structures and therefore exhibit layer- and timestep-wise characteristics that are largely consistent with those observed in SD~2.1 (\cref{fig:another_backbone_freq}~(d)). 
% Based on this observation, applying CHIMERA leads to consistent performance improvements across these models, as reported in \cref{tab:backbone_comparison}.

% As shown in \cref{fig:another_backbone_freq}~(e), SDXL exhibits frequency characteristics similar to those of SD~2.1, although the number of layers differs from that of SD~2.1. 
% To further demonstrate that CHIMERA is not limited to U-Net-based architectures, we extend the analysis to the diffusion transformer model FLUX (\cref{fig:another_backbone_freq}~(f)). 
% As noted in prior DiT-based studies~\cite{chang2025sparsedit, yu2024representation}, early layers of DiT mainly capture low-frequency components, while later layers focus on high-frequency details; similarly, early timesteps tend to generate low-frequency structures, while later timesteps refine high-frequency details. 
% These properties are also reflected in \cref{fig:another_backbone_freq}~(f). Based on these observations, applying CHIMERA to both SDXL and FLUX results in consistent performance improvements, as shown in \cref{tab:backbone_comparison}. 
% These results demonstrate that CHIMERA is not limited to a specific backbone and can be effectively extended to a wide range of diffusion-based models.
